# Supplementary material for: DreamHMR: From Video Generation to Human Motion Modeling via Structural Focusing
Source: arXiv:2610.20124 source file (2026-10-14)
Supplement: Supplementary file 5 [file impro.tex]

\begin{figure}[p]
\centering
{\expfloatstyle
\setlength{\tabcolsep}{2pt}
\textbf{Figure~\ref{fig:app-four-dips} (continued)}\par\medskip
\textbf{(o) 2.67 s}\par\smallskip
\begin{tabular}{@{}cccc@{}}
RGB & Hand4Whole++ & SMPLest-X & GT \\[2pt]
\includegraphics[width=.238\linewidth,height=.168\textheight,keepaspectratio]{figures/appendix-comparison/impro-0080-rgb.jpg} & \includegraphics[width=.238\linewidth,height=.168\textheight,keepaspectratio]{figures/appendix-comparison/impro-0080-hand4whole.jpg} & \includegraphics[width=.238\linewidth,height=.168\textheight,keepaspectratio]{figures/appendix-comparison/impro-0080-smplest.jpg} & \includegraphics[width=.238\linewidth,height=.168\textheight,keepaspectratio]{figures/appendix-comparison/impro-0080-gt.jpg} \\[4pt]
\textcolor{expteal}{\textbf{Wan-1.3B}} & \textcolor{expteal}{\textbf{Wan-5B}} & \textcolor{expteal}{\textbf{LTX-2B}} & \textcolor{expteal}{\textbf{Cosmos-2B}} \\[2pt]
\includegraphics[width=.238\linewidth,height=.168\textheight,keepaspectratio]{figures/appendix-comparison/impro-0080-Wan-1.3B.jpg} & \includegraphics[width=.238\linewidth,height=.168\textheight,keepaspectratio]{figures/appendix-comparison/impro-0080-Wan-5B.jpg} & \includegraphics[width=.238\linewidth,height=.168\textheight,keepaspectratio]{figures/appendix-comparison/impro-0080-LTX-2B.jpg} & \includegraphics[width=.238\linewidth,height=.168\textheight,keepaspectratio]{figures/appendix-comparison/impro-0080-Cosmos-2B.jpg} \\[4pt]
\end{tabular}\par\medskip
\textbf{(p) 6.67 s}\par\smallskip
\begin{tabular}{@{}cccc@{}}
RGB & Hand4Whole++ & SMPLest-X & GT \\[2pt]
\includegraphics[width=.238\linewidth,height=.168\textheight,keepaspectratio]{figures/appendix-comparison/impro-0200-rgb.jpg} & \includegraphics[width=.238\linewidth,height=.168\textheight,keepaspectratio]{figures/appendix-comparison/impro-0200-hand4whole.jpg} & \includegraphics[width=.238\linewidth,height=.168\textheight,keepaspectratio]{figures/appendix-comparison/impro-0200-smplest.jpg} & \includegraphics[width=.238\linewidth,height=.168\textheight,keepaspectratio]{figures/appendix-comparison/impro-0200-gt.jpg} \\[4pt]
\textcolor{expteal}{\textbf{Wan-1.3B}} & \textcolor{expteal}{\textbf{Wan-5B}} & \textcolor{expteal}{\textbf{LTX-2B}} & \textcolor{expteal}{\textbf{Cosmos-2B}} \\[2pt]
\includegraphics[width=.238\linewidth,height=.168\textheight,keepaspectratio]{figures/appendix-comparison/impro-0200-Wan-1.3B.jpg} & \includegraphics[width=.238\linewidth,height=.168\textheight,keepaspectratio]{figures/appendix-comparison/impro-0200-Wan-5B.jpg} & \includegraphics[width=.238\linewidth,height=.168\textheight,keepaspectratio]{figures/appendix-comparison/impro-0200-LTX-2B.jpg} & \includegraphics[width=.238\linewidth,height=.168\textheight,keepaspectratio]{figures/appendix-comparison/impro-0200-Cosmos-2B.jpg} \\[4pt]
\end{tabular}\par\medskip
}
\end{figure}
